# Supplementary material for: Instant3D: Fast Text-to-3D with Sparse-View Generation and Large Reconstruction Model
Source: arXiv:2311.06214 source file (2023-11-23)
Supplement: Supplementary file 1 [file appendix_curated_vs_random.tex]

\begin{figure}
\includegraphics[width=\textwidth]{figures/appendix/appendix_curated_vs_random.pdf}
\vspace{-0.5cm}
\caption{
Comparison on generated 2x2 grid images with SDXL models fine-tuned with  
\sai{XX} curated data and random data. We can see that the model trained 
with curated data generates images with more geometric and texture details as 
well as better photo realism. 
}
\label{fig:appendix-curated-vs-random}
\end{figure}
