# Supplementary material for: Instant3D: Fast Text-to-3D with Sparse-View Generation and Large Reconstruction Model
Source: arXiv:2311.06214 source file (2023-11-23)
Supplement: Supplementary file 2 [file uncurated_baseline_comp.tex]

\begin{figure}
\vspace{-1cm}
\includegraphics[width=\textwidth]{figures/appendix/uncurated_comparison/instant3d_uncurated_comp_Part1.pdf}
\vspace{-0.4cm}
\caption{
Uncurated comparison between Shap-E, DreamFusion, ProlificDreamer and our method. The prompts used in this figure are:
(A) a t-rex roaring up into the air
(B) a corgi wearing a top hat
(C) an orc forging a hammer on an anvil
(D) a chimpanzee stirring a bubbling purple potion in a cauldron
(E) a wedge of cheese on a silver platter
(F) an iguana holding a balloon
(G) a frog wearing a sweater
(H) a group of squirrels rowing crew
(I) an astronaut chopping vegetables in a sunlit kitchen
(J) the titanic, aerial view
(K) a barbecue grill cooking sausages and burger patties
(L) a wooden desk and chair from an elementary school.
Inference time: Shap-E (6 seconds), DreamFusion (1.5 hours), ProlificDreamer (10 hours), and Ours (20 seconds). 
}
\label{fig:uncurated_comparison}
\end{figure}
